# Supplementary material for: An investigation of GPU-based stiff chemical kinetics integration methods
Source: arXiv:1607.03884 ancillary file (2017-02-14)
Supplement: Supplementary file 1 [file GPU-integrator-supplementary-material.pdf]

# Supplementary material for "An investigation of GPU-based stiff chemical kinetics integration methods"

Nicholas J. Curtis*[1], Kyle E. Niemeyer[2], and Chih-Jen Sung[1]

[1]Department of Mechanical Engineering, University of Connecticut, Storrs, CT, USA

[2]School of Mechanical, Industrial, and Manufacturing Engineering, Oregon State University, Corvallis, OR, USA

## 1 Raw performance plots

In this section we present the plots of the raw, unnormalized performance data for completeness, as described in Sec. 3. Figures 1 and 2 show performance for the hydrogen and GRI-Mech 3.0 models, respectively.

*Email: nicholas.curtis@uconn.edu

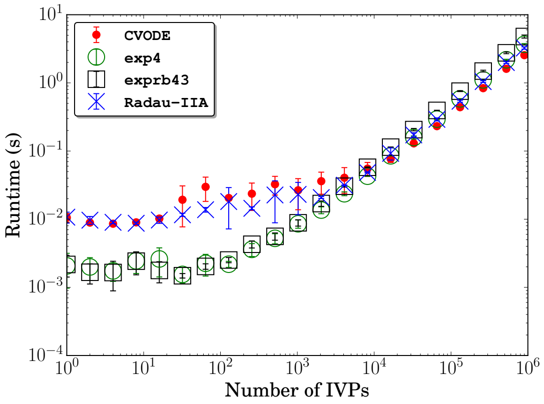


(a) CPU performance results for $\Delta t = 10^{-6}$ s

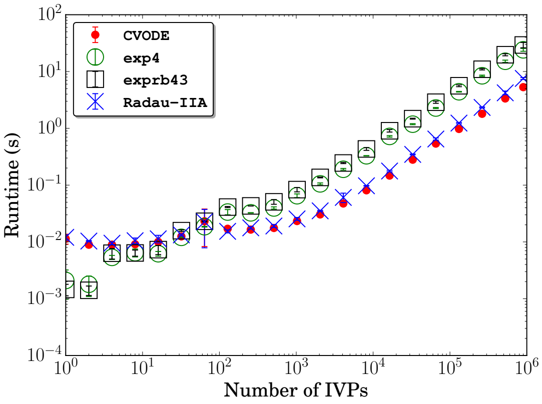


(b) CPU performance results for $\Delta t = 10^{-4}$ s

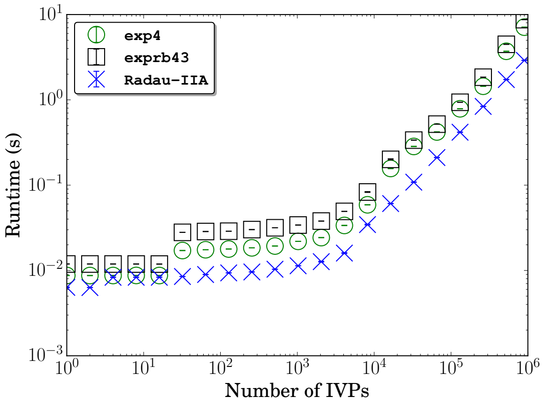


(c) GPU performance results for $\Delta t = 10^{-6}$ s

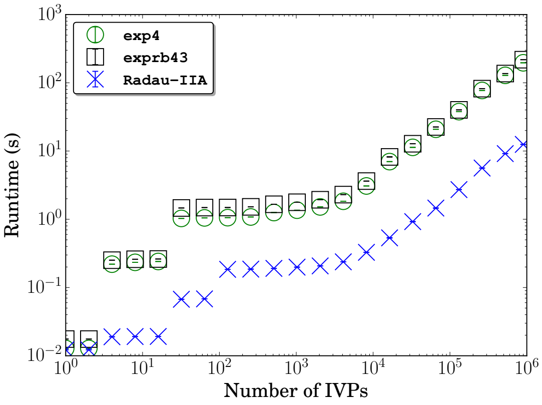


(d) GPU performance results for $\Delta t = 10^{-4}$ s

Figure 1: Average (unnormalized) runtimes of the integrators on the CPU and GPU for the hydrogen model at two different global time-step sizes. Error bars indicate standard deviation. Data, plotting scripts, and figure files available under CC-BY [1].

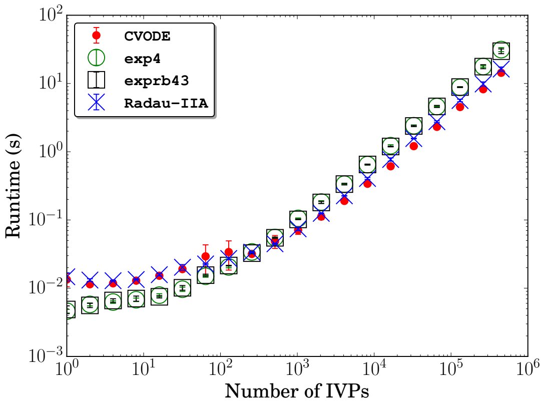


(a) CPU performance results for $\Delta t = 10^{-6}$ s

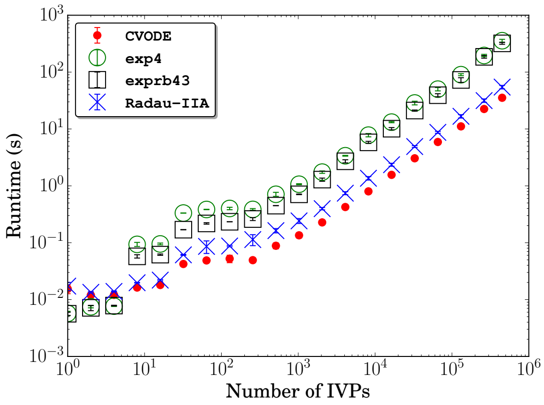


(b) CPU performance results for $\Delta t = 10^{-4}$ s

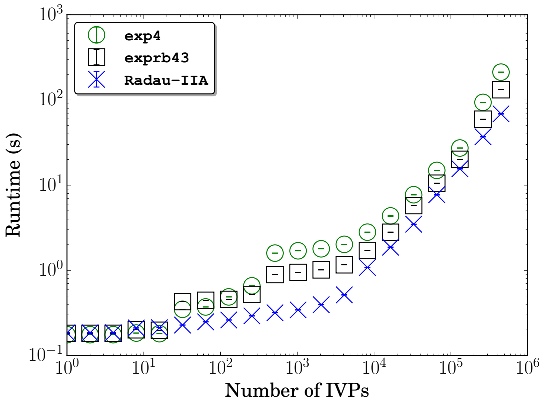


(c) GPU performance results for $\Delta t = 10^{-6}$ s

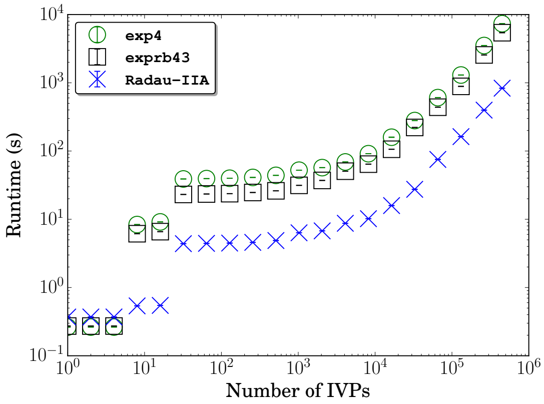


(d) GPU performance results for $\Delta t = 10^{-4}$ s

Figure 2: Average (unnormalized) runtimes of the integrators on the CPU/GPU for the GRI-Mech 3.0 model at two different global time-step sizes. Error bars indicate standard deviation. Data, plotting scripts, and figure files available under CC-BY [1].

## 2 Characterization of partially stirred reactor data

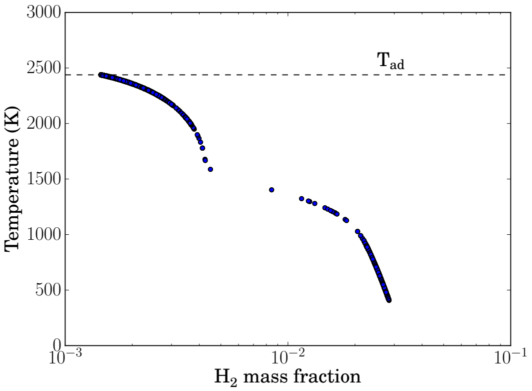


(a) Temperature/$H_2$ mass fraction distribution for a hydrogen run.

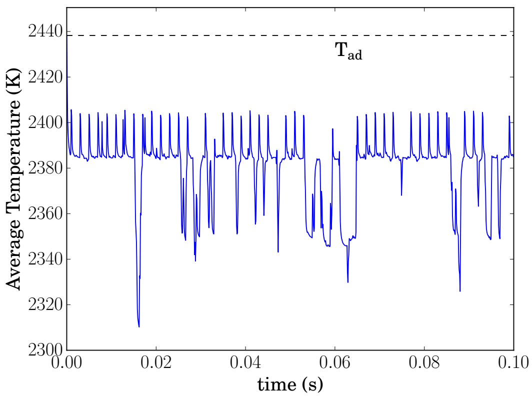


(b) Average temperature in the PaSR for hydrogen run.

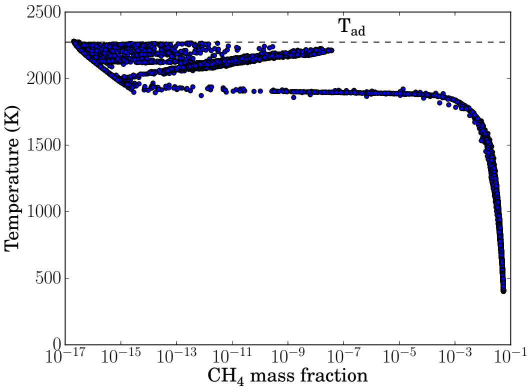


(c) Temperature/$CH_4$ mass fraction distribution for a GRI-Mech 3.0 run.

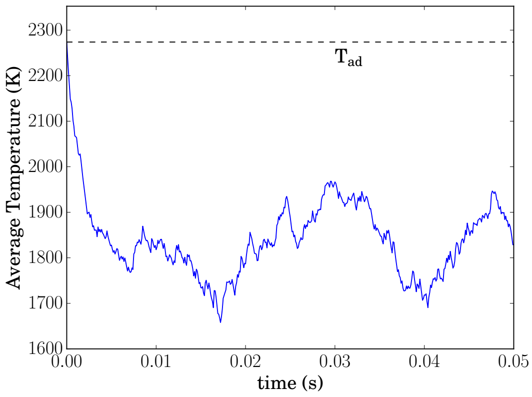


(d) Average temperature in the PaSR for a GRI-Mech 3.0 run.

Figure 1: Characterizations of the conditions sampled from the PaSR at 400 K, 1 atm for both models. The adiabatic flame temperature $T_{ad}$ is by a dashed line in all cases. Data, plotting scripts, and figure files available under CC-BY [1].

Figure 1 shows a characterization example of the PaSR conditions sampled for validation and performance testing in this work; a wide range of temperatures and fuel-mass fractions are observed for both models. Significantly more diversity in fuel mass-fraction is seen for the GRI-Mech 3.0 near the adiabatic flame temperature. Further, the hydrogen model is more sensitive to the mixing/pairing time-scales, showing many large temperature changes quickly recovering to a semi-stable temperature. The databases used in this work are

available online [2, 3].

## References


[1] NJ Curtis, KE Niemeyer, and CJ Sung. *Data, plotting scripts, and figures for "An investigation of GPU-based stiff chemical kinetics integration methods"*. figshare, CC-BY license. 2017. DOI: `10.6084/m9.figshare.4596847`.

[2] NJ Curtis and KE Niemeyer. *h2_pasr_data.bin*. figshare. Oct. 2016. DOI: `10.6084/m9.figshare.4007427.v3`.

[3] NJ Curtis and KE Niemeyer. *ch4_pasr_data.bin*. figshare. Oct. 2016. DOI: `10.6084/m9.figshare.4007418.v2`.
